# Supplementary material for: Logarithmic Spatial Variations and Universal $f^{-1}$ Power Spectra of Temperature Fluctuations in Turbulent Rayleigh-B\'enard Convection
Source: arXiv:1405.0432 source file (2014-05-02)
Supplement: Supplementary file 1 [file Supplement.pdf]

# Supplement to “Logarithmic spatial variations and universal $f^{-1}$ power spectra of temperature fluctuations in turbulent Rayleigh-Bénard convection” by He *et al.*

February 25, 2014

## 1 The “elliptic approximation” and the equivalence between the space and time domain

The elliptic approximation (EA) of He and Zhang [1, 2] was first formulated for the velocity correlation functions of turbulent shear flows. In the bulk of turbulent Rayleigh-Bénard convection temperature has been shown to behave as a passive scalar [3, 4]; thus its temperature correlation functions to an excellent approximation are the same as those of the velocity field and we shall formulate the EA in terms of the temperature field.

It will become apparent that the EA is a **systematic** approximation since it is an **exact** expansion of the correlation function to second order in space and time. The only way in which the EA and its consequences could deviate from the complete result is *via* fourth and higher order terms (odd terms vanish because of homogeneity and stationarity), which are believed to be small.

The EA includes the influence of both the mean-flow velocity  $U$  and a root-mean-square fluctuation velocity  $V$ . We shall see that, in the limit as  $V$  vanishes, the EA reduces to the Taylor frozen-flow approximation.

### 1.1 The approximation

From the temperature as a function of position and time one can calculate the temperature space-time cross-correlation function

$$C(l, \tau) = \langle \delta T(x + l, t + \tau) \delta T(x, t) \rangle / (\sigma_x \sigma_{x+l}) . \quad (1)$$

Here  $\langle \dots \rangle$  denotes the time average,  $\delta T = T(t) - \langle T \rangle$ , and  $\sigma_x$  and  $\sigma_{x+l}$  are the rms values of  $\delta T$  at the vertical positions  $x$  and  $x + l$ . In homogeneous and isotropic turbulent flows temperature space-time cross-correlation functions  $C(l, \tau)$  can be described well by the elliptic approximation (EA) developed by He and Zhang

[1] and Zhao and He [2]. For  $l$  and  $\tau$  close to 0, the Taylor-series expansion of  $C(l, \tau)$  has the form

$$\begin{aligned} C(l, \tau) = & C(0, 0) + \frac{\partial C(0, 0)}{\partial l} l + \frac{\partial C(0, 0)}{\partial \tau} \tau + \frac{\partial^2 C(0, 0)}{\partial l \partial \tau} l \tau \\ & + \frac{1}{2} \left[ \frac{\partial^2 C(0, 0)}{\partial l^2} l^2 + \frac{\partial^2 C(0, 0)}{\partial \tau^2} \tau^2 \right] + \dots \end{aligned} \quad (2)$$

For a spatially homogeneous and statistically stationary process, the odd derivatives on the rhs of Eq. 2 vanish. The elliptic approximation consists of truncating Eq. 2 at second order; thus corrections to the EA will be of fourth and higher order. The terms up to second order can be written as

$$\begin{aligned} C(l, \tau) &= C(0, 0) + \frac{1}{2} \frac{\partial^2 C(0, 0)}{\partial l^2} l_E^2 \\ &= C(l_E, 0), \end{aligned} \quad (3)$$

where the rescaled space separation  $l_E$  is given by

$$l_E^2 = (l - U\tau)^2 + (V\tau)^2 \quad (4)$$

and where the two velocities  $U$  and  $V$  are

$$U = - \frac{\partial^2 C(0, 0)}{\partial l \partial \tau} \left[ \frac{\partial^2 C(0, 0)}{\partial l^2} \right]^{-1} \quad (5)$$

and

$$V = - \frac{\partial^2 C(0, 0)}{\partial \tau^2} \left[ \frac{\partial^2 C(0, 0)}{\partial l^2} \right]^{-1}. \quad (6)$$

Both the EA velocities can be derived [1] from the Boussinesq equations. The velocity  $U$  is the component of the mean flow velocity along the  $l$  direction, *i.e.*  $U = \langle U(t) \rangle_t$ . The other velocity  $V$  is determined by the rms velocity  $v_0$  and a shear-induced contribution [2]. The shear contribution was estimated to be negligibly small for RBC [5], so that one may take  $V = v_0$ . Then we have  $V = \langle (U(t) - U)^2 \rangle^{1/2}$ .

We note that Eq. 3 implies that a constant  $l_E$  implies that  $C(l, \tau)$  is constant. Further, constant  $l_E$  corresponds to an elliptic contour in the  $l, \tau$  plane as shown in Fig. 1. Thus, any such contour, in addition to corresponding to a constant  $l_E$ , also is a contour of constant correlation.

In the absence of fluctuations (*i.e.*  $V = 0$ ) Eq. 4 reduced to

$$l = l_E + U\tau \quad (7)$$

which corresponds to the Taylor frozen-flow hypothesis. Thus, the Taylor hypothesis is represented by a straight line with slope equal to  $U$  and intercept  $l = l_E$  in Fig. 1.

The second-order expansion Eq. 2 is valid for small  $l$  and  $\tau$  with the next correction terms being of fourth order. He and Zhang [1, 2] argued that the EA

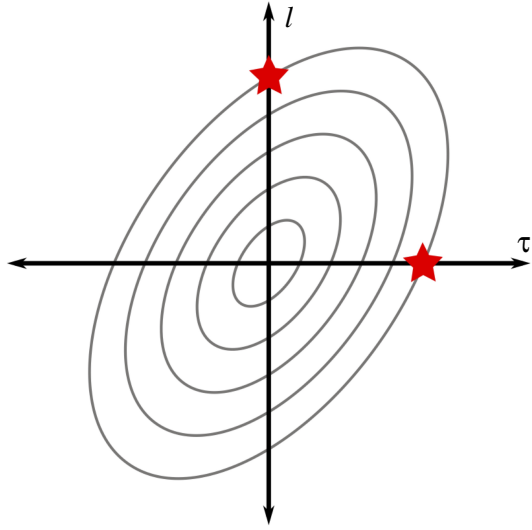

Figure 1: Contours of constant  $l_E$  and constant correlation in the  $l - \tau$  plane.

represented by Eqs. (3) and (4) is also valid for larger values of  $l$  and  $\tau$  if the flow is scale invariant as it is expected to be in the inertial range, *i.e.* when the Reynolds number is sufficiently large. In this case, all the iso-correlation contours of  $C(l, \tau)$  for large  $l$  and  $\tau$  are also expected to be elliptic and to have shapes like those shown in Fig. 1. The justification of the similarity assumption for correlation contours was based on Kolmogorov's self-similarity hypothesis [6] for turbulent flows. Using direct numerical simulation (DNS) data for turbulent channel flows, He and Zhang [1] verified the similarity assumption for correlation contours and tested the EA successfully in turbulent shear flows. In experiment, the similarity assumption and the EA method had been found valid for both temperature [5, 7] and velocity [8] measurements in a  $\Gamma = 1$  RBC sample for  $\text{Pr} \simeq 4.3$  and  $\text{Ra} \simeq 10^{10}$ . For our sample we carried out extensive tests (to be reported elsewhere) and showed that the EA was valid over spatial and temporal ranges much larger than any used in the present work.

## 1.2 The equivalence between the space and time domain

The equation

$$l = V_{eff}\tau \quad (8)$$

cited in our main document follows from Eq. 4 which is also Eq. (8) of [1]. Let us consider the special cases  $(l = 0, \tau)$  and  $(l, \tau = 0)$  as indicated by the stars in Fig. 1. For  $l = 0$   $l_E$  reduces to  $l_{E,l=0} = \sqrt{U^2 + V^2}\tau$ , while for  $\tau = 0$  we have  $l_{E,\tau=0} = l$ . Since the ellipses are constant-correlation contours, we have

$$C(l, 0) = C(0, \tau) \quad (9)$$

provided  $l_{E,l=0} = l_{E,\tau=0}$  or

$$l = \sqrt{U^2 + V^2} * \tau = V_{eff} * \tau \quad (10)$$

which is Eq. 8.

For  $l$  or  $\tau$  close to 0, we defined the length scale  $\lambda_0$  or the time scale  $\tau_0$  by

$$C(l, 0) = 1 - (l/\lambda_0)^2 + \dots \quad (11)$$

and

$$C(0, \tau) = 1 - (\tau/\tau_0)^2 + \dots \quad (12)$$

Using Eq. 9 with Eq. 11 and Eq. 12 gives

$$l/\lambda_0 = \tau/\tau_0 \quad (13)$$

With Eq. 10 this gives

$$\lambda_0 = V_{eff} * \tau_0 \quad (14)$$

and thus the equivalence

$$C(l/\lambda_0, 0) = C(0, \tau/\tau_0) \quad (15)$$

between the space and time domain. Fourier transforming Eq. 15 yields the corresponding equivalence

$$E(k\lambda_0) = P(f\tau_0) \quad (16)$$

in the wavenumber and frequency space.

## 2 Experimental details and tests

### 2.1 Thermometer response

The measurements of correlation functions and spectra require that the temperature sensors have a sufficiently fast time response and that the time series taken are of sufficient length, time resolution, and temperature resolution.

In order to address the first of these issues, we compared the results from three thermistors of different sizes and thus response times. Photographs of the sensors are shown in Fig. 2(a). We used primarily the middle sized thermistors  $T_2$  which had a diameter of  $360 \mu\text{m}$ . According to the comparison in Fig. 2 with the even smaller thermistor  $T_3$  it has no loss of power for frequencies less than 0.5 Hz and even for higher frequencies produces a near-perfect spectrum. The range of the  $f^{-1}$  form of the spectra was limited to  $f \lesssim 0.2$  Hz at all Rayleigh numbers. Thus in the frequency range of interest we are confident that there is no spectral distortion due to finite response time of the sensor.

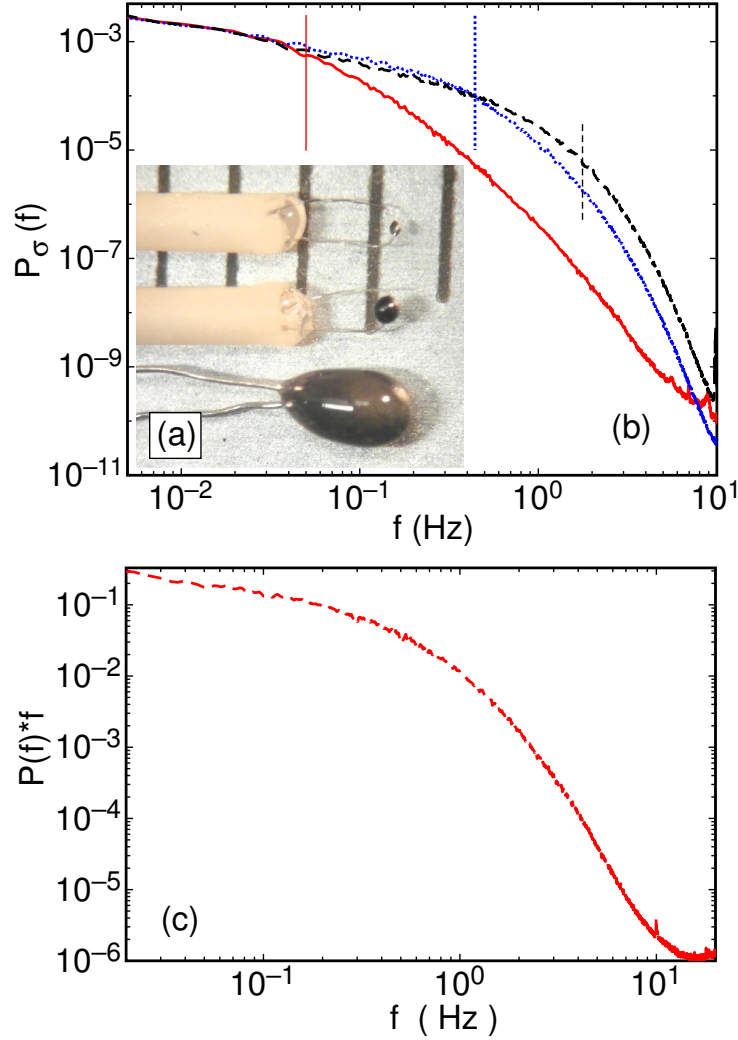

Figure 2: (a): A picture of the three thermistor types used in this work. The scale shown for comparison has marks at intervals of 1 mm. (b): Power spectra  $P_\sigma$  of  $\delta T/\Delta T$  for the three types of thermistors ( $\delta T = T(t) - \langle T(t) \rangle_t$  and  $\Delta T$  is the applied temperature difference). Dashed (black) line:  $T_3$  with  $d = 0.18$  mm. Dotted (blue) line:  $T_2$  with  $d = 0.36$  mm. Solid (red) line:  $T_1$  with  $d = 1.13$  mm. All were located 4.1 cm from the top or bottom plate and 1.0 cm from the side wall, and  $Ra = 1.05 \times 10^{15}$ . The short vertical lines indicate our estimates of the frequency  $f_c$  below which the spectrum is unattenuated by the thermistor size. (c): Normalized temperature power spectrum  $P(f)$ , compensated by the frequency  $f$  in Hz, as a function of  $f$  for  $z/L = 0.4933$ ,  $Ra = 1.08 \times 10^{15}$ ,  $(R-r)/D = 0.0178$ . Please note that  $P_\sigma(f)$  in (b) is not the same quantity as  $P(f)$  in (c).

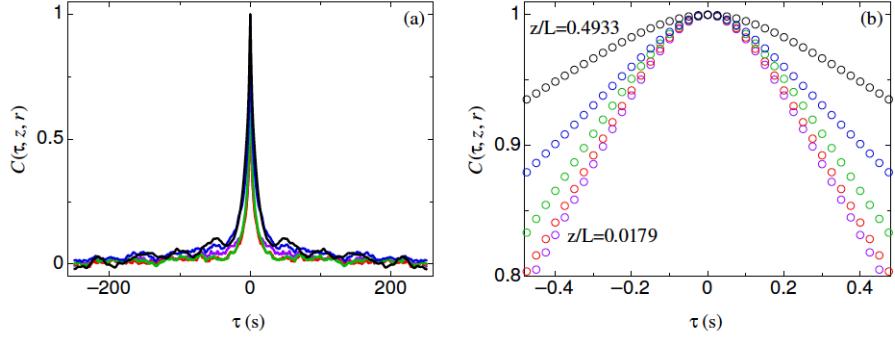

Figure 3: (a): Auto-correlation functions  $C(\tau, z, r)$  as a function of  $\tau$  measured from thermistors at the radial position  $(R - r)/D = 0.0178$  for various vertical positions  $z/L = 0.0179$  (purple), 0.0362 (red), 0.0719 (green), 0.1437 (blue) and 0.4933 (black). (b) The same  $C(\tau, z, r)$  data as in (a), but only near the origin of  $\tau$ .

## 2.2 Spectral measurements

For all our time series we typically discarded initial data for several hours in order to avoid transients. Then we typically collected data for 15 hours at a rate of 40 Hz, thus yielding about  $2.2 \times 10^6$  data points. Spectra and correlation functions were computed using all  $2.2 \times 10^6$  points. From the spectrum in Fig. 2(c) one sees clearly that the Nyquist frequency  $f_N$  is in the frequency range where only background noise contributes. That noise level is about seven orders of magnitude below the power at low frequencies. Thus any contribution from frequencies above  $f_N$  are too feeble to cause any noticeable distortion of the spectrum below  $f_N$ .

## 2.3 Correlation functions

In Fig. 3(a) we show several correlation functions taken at various vertical positions. They decay to zero for  $|\tau| \gtrsim 100$  or 200 s as they should in the absence of drift or slow transients in the data. Figure 3(b) shows the same data as (a), but only over the narrow time interval  $|\tau| < 0.5$  s. The data shown in Fig. 2(a) of the main document are the uppermost set, for  $z/L = 0.493$ , and a parabola fits the data near the peak, for  $C(\tau) \gtrsim 0.995$  and  $|\tau| \lesssim 0.1$  s, extremely well.

## References

- [1] G.-W. He and J.-B. Zhang, *Elliptic model for space-time correlations in turbulent shear flows*, Phys. Rev. E **73**, 055303 (2006).

- [2] X. Zhao and G.-W. He, *Space-time correlations of fluctuating velocities in turbulent shear flows*, Phys. Rev. E **79**, 046316 (2009).
- [3] C. Sun, Q. Zhou, and K. Q. Xia, *Cascades of velocity and temperature fluctuations in buoyancy-driven thermal turbulence*, Phys. Rev. Lett. **97**, 144504 (2006).
- [4] X. He, E. S. C. Ching, and P. Tong, *Locally averaged thermal dissipation rate in turbulent thermal convection: A decomposition into contributions from different temperature gradient components*, Phys. of Fluids **23**, 1 (2011).
- [5] X. He, G. He, and P. Tong, *Small-scale turbulent fluctuations beyond Taylors frozen-flow hypothesis*, Phys. Rev. E **81**, 065303 (2010).
- [6] A. N. Kolmogorov, CR. Acad. Sci. USSR. **30**, 299 (1941).
- [7] X. He and P. Tong, *Kraichnans random sweeping hypothesis in homogeneous turbulent convection*, Phys. Rev. E **83**, 037302 (2011).
- [8] Q. Zhou, C.-M. Li, Z.-M. Lu, and Y.-L. Liu, *Experimental investigation of longitudinal space-time correlations of the velocity field in turbulent Rayleigh-Bénard convection*, J. Fluid Mech. **683**, 94 (2011).
